# Supplementary material for: Network Meta Analysis of Mean Survival
Source: arXiv:2512.09732 source file (2025-12-10)
Supplement: Supplementary file 1 [file supplement.pdf]

# Supplementary Materials for Synthesis of mean survival times for cost-effectiveness analyses by Anastasios Apsemidis, Dimitris Mavridis and Nikolaos Demiris

Anastasios Apsemidis[1], Dimitris Mavridis[2], Nikolaos Demiris[3]

[1]Department of Primary Education, University of Ioannina, Ioannina, Greece, a.apsemidis@uoi.gr
[2]Department of Primary Education, University of Ioannina, Ioannina, Greece, dmavridi@uoi.gr
[2]Department of Statistics, Athens, University of Economics and Business, Greece, nikos@aueb.gr

# Web Appendix A. Details on the NMA model

In the main text, we described the second level of the NMA hierarchy using the conditional distributions of the random effects:

$$\delta_{j,k} \sim N\left(\nu_{T_{j,k}}, \frac{k}{2(k-1)}\tau^2\right)$$
$$\nu_{T_{j,k}} = d_{T_{j,k}} - d_{T_{j,1}} + \frac{1}{k-1}\sum_{w=1}^{k-1}(\delta_{j,w} - d_{T_{j,w}} + d_{T_{j,1}})$$

This implies the multivariate structure

$$\begin{pmatrix} \delta_{j,2} \\ \delta_{j,3} \\ \vdots \\ \delta_{j,A_j} \end{pmatrix} \sim \mathbf{N}_{A_j-1}\left[\begin{pmatrix} d_{T_{j,2}} - d_{T_{j,1}} \\ d_{T_{j,3}} - d_{T_{j,1}} \\ \vdots \\ d_{T_{j,A_j-1}} - d_{T_{j,1}} \end{pmatrix}, \begin{pmatrix} \tau^2 & \tau^2/2 & ... & \tau^2/2 \\ \tau^2/2 & \tau^2 & ... & \tau^2/2 \\ \vdots & \vdots & ... & \vdots \\ \tau^2/2 & \tau^2/2 & ... & \tau^2 \end{pmatrix}\right]$$

where each $\delta_{j,k}$ is the true study-specific effect of treatment $T_{j,k}$ relative to $T_{j,1}$. When we have multiple arms in a single study, the random effects for the different contrasts are not independent (within the study). They are correlated, because all contrasts share the same baseline arm and, so treating them as independent would contribute too much information. This is the reasoning behind the multi-arm correction. In practice, one can use either the conditional, or the multivariate formulation and, in the melanoma example (which includes a 3-arm trial) we test the STAN models using either one (see Web Appendix E).

Thus, in practice, one may use a more compact notation for the LYG NMA model:

$$\mathbf{y}_j|\boldsymbol{\delta}_j \sim \mathbf{N}_{A_j-1}(\boldsymbol{\delta}_j, \Sigma_{obs,j}) \quad (1)$$

$$\boldsymbol{\delta}_j|\mathbf{d}, \tau^2 \sim \mathbf{N}_{A_j-1}(\mu_j(\mathbf{d}), \Sigma_{between,j}(\tau^2)) \quad (2)$$

where $\mathbf{y}_j$ can be either a scalar (2-arm case), or a vector of contrasts (multi-arm case) and $\boldsymbol{\delta}_j$ is the vector of $\delta_{j,2}$, $\delta_{j,3}$, ..., $\delta_{j,A_j}$. For each arm $k \geq 2$, $\mu_{j,k}(d) = d_{T_{j,k}} - d_{T_{j,1}}$, while for

the variance terms: $\Sigma_{obs,j}[k,k] = \sigma^2_{j,k}$, $\Sigma_{pbs,j}[k,l] = s_{j,1}$ (for $k \neq l$), $\Sigma_{between,j}[k.k] = \tau^2$ and $\Sigma_{between,j}[k,l] = \tau^2/2$ (for $k \neq l$).

# Web Appendix B. Decision theoretic implementations using MCMC

Here, we explain how a practitioner can apply the decision theoretic framework for meta-analysis using posterior draws from LYG estimates (for NMA using absolute effects, the parameter space changes to one containing the relevant quantities, but everything else remain the same). We have estimated a posterior over LYG between treatment comparisons $p(\theta|x)$ via $S$ Markov Chain Monte Carlo (MCMC) draws, i.e. we have $\theta^{(1)}, ..., \theta^{(S)}$, with $\theta^{(s)} = (d_1^{(s)}, ..., d_K^{(s)})$. The posterior risk $PR(\theta, \delta(\mathbf{x}))$ is the expected loss after choosing treatment $k$ (given data), i.e.

$$\mathbb{E}_{\theta|\mathbf{x}} L(\theta, a_k) = \frac{1}{S} \sum_{s=1}^{S} L(\theta^{(s)}, a_k) \tag{3}$$

Minimizing the sum for each draw $s$ among the available treatments yields a distribution over the Bayes risk and the minimizer at each draw is the Bays rule.

We consider three loss functions (apart from LaEV, mentioned in the main text), namely the 0-1, the regret, and the squared regret. The 0-1 loss is defined as

$$L_{01}(\theta, a_k) = \begin{cases} 0 & \text{if } a_k = \max_k d_k \\ 1 & \text{otherwise} \end{cases} \tag{4}$$

Minimizing the posterior risk under the 0-1 loss leads to picking the treatment with largest

probability of being best and this can be seen writing:

$$\begin{aligned} PR(\theta, \delta(\mathbf{x})) &= \mathbb{E}_{\theta|\mathbf{x}} L_{01}(\theta, a_k) \\ &= \int_{\Theta} L_{01}(\theta, a_k) p(\theta|\mathbf{x}) d\theta \\ &= P(\{a_k \neq \max_k d_k|\mathbf{x}\}) = 1 - P(\{a_k = \max_k d_k|\mathbf{x}\}) \end{aligned}$$

Thus, minimization of the posterior risk over treatments leads to maximization of the posterior probability of treatment $k$ being the maximizer. In practice, for each treatment $k$, we compute the average number of times each treatment ranks first, $\frac{1}{S}\sum_{s=1}^{S} I(a_k^{(s)} = \max_k d_k^{(s)})$, and the Bayes rule is the treatment with the largest such value.

On the other hand, the linear regret loss is defined as $L_{reg}(\theta, a_k) = \max_k d_k - a_k$, so the posterior risk reads:

$$\begin{aligned} PR(\theta, \delta(\mathbf{x})) &= \mathbb{E}_{\theta|\mathbf{x}} L_{reg}(\theta, a_k) \\ &= \mathbb{E}[\max_k d_k - a_k] \\ &= \mathbb{E}[\max_k d_k|\mathbf{x}] - \mathbb{E}[a_k|\mathbf{x}] \end{aligned}$$

so minimizing the posterior risk over treatments is equivalent to maximizing the posterior mean $\mathbb{E}[a_k|\mathbf{x}]$. Using MCMC samples, we can calculate the average LYG over draws for each treatment, $\frac{1}{S}\sum_{s=1}^{S} a_k^{(s)}$, and select the treatment with the highest value. For the squared regret, we get the maximum LYG over draws, $\frac{1}{S}\sum_{s=1}^{S} \max_k d_k^{(s)}$, subtract the average LYG over draws per treatment, $\frac{1}{S}\sum_{s=1}^{S} a_k^{(s)}$, and simply square the result.

# Web Appendix C. Power-likelihood simulation study

| $n_{bad}$ | Bias added | NMA | Bias | RMSE | Coverage | CrI width | Variance |
|---|---|---|---|---|---|---|---|
| 2 | 0.0 | power | -0.050 | 0.149 | 1.000 | 0.529 | 0.018 |
| 4 | 0.0 | power | 0.063 | 0.162 | 1.000 | 0.536 | 0.020 |
| 6 | 0.0 | power | 0.083 | 0.173 | 1.000 | 0.498 | 0.016 |
| 2 | 0.5 | power | -0.045 | 0.145 | 1.000 | 0.505 | 0.016 |
| 4 | 0.5 | power | 0.058 | 0.167 | 1.000 | 0.588 | 0.024 |
| 6 | 0.5 | power | -0.264 | 0.295 | 0.500 | 0.505 | 0.016 |
| 2 | 1.0 | power | 0.118 | 0.229 | 1.000 | 0.645 | 0.027 |
| 4 | 1.0 | power | 0.094 | 0.189 | 1.000 | 0.623 | 0.025 |
| 6 | 1.0 | power | 0.049 | 0.199 | 1.000 | 0.715 | 0.034 |
| 2 | 0.0 | typical | -0.013 | 0.147 | 1.000 | 0.557 | 0.020 |
| 4 | 0.0 | typical | 0.057 | 0.157 | 1.000 | 0.516 | 0.019 |
| 6 | 0.0 | typical | 0.064 | 0.157 | 1.000 | 0.493 | 0.016 |
| 2 | 0.5 | typical | -0.041 | 0.167 | 1.000 | 0.585 | 0.022 |
| 4 | 0.5 | typical | 0.036 | 0.178 | 1.000 | 0.635 | 0.027 |
| 6 | 0.5 | typical | -0.322 | 0.352 | 0.333 | 0.535 | 0.019 |
| 2 | 1.0 | typical | 0.126 | 0.258 | 1.000 | 0.753 | 0.037 |
| 4 | 1.0 | typical | 0.124 | 0.232 | 1.000 | 0.741 | 0.035 |
| 6 | 1.0 | typical | 0.076 | 0.227 | 1.000 | 0.784 | 0.041 |

Table 1: Simulation results for each scenario of number of 'bad' studies ($n_{bad}$, added bias level and mean metrics regarding estimation of treatment effects: bias, RMSE, coverage, CrI width, and posterior variance. The values are rounded to 3 decimal digits. The corresponding Figure lies in the main text.

# Web Appendix D. Results on the sampler comparison

The results of the simulation study regarding estimation of treatment differences (the $d$ parameters) are gathered here per scenario and engine. The scenarios tested are given in Table 2. For each scenario and engine we compute the statistical metrics bias, RMSE, MAE, coverage, credible interval width, WAIC, LOO, logS, CRPS and the computational metrics ESS, ESS per second, runtime, iterations per second, parameter draws per second and number of divergent transitions.

Table 2: Simulation scenarios by heterogeneity level ($\sigma$), number of treatments ($n_t$), and number of studies ($n_s$). Labels are updated by this specific order.

| Between-study sd | Number of treatments | Number of studies | | |
|---|---|---|---|---|
| | | $n_s = 7$ | $n_s = 20$ | $n_s = 50$ |
| $sd = 0.1$ | $n_t = 4$ | Scenario 1 | Scenario 7 | Scenario 13 |
| | $n_t = 8$ | Scenario 4 | Scenario 10 | Scenario 16 |
| $sd = 0.3$ | $n_t = 4$ | Scenario 2 | Scenario 8 | Scenario 14 |
| | $n_t = 8$ | Scenario 5 | Scenario 11 | Scenario 17 |
| $sd = 1$ | $n_t = 4$ | Scenario 3 | Scenario 9 | Scenario 15 |
| | $n_t = 8$ | Scenario 6 | Scenario 12 | Scenario 18 |

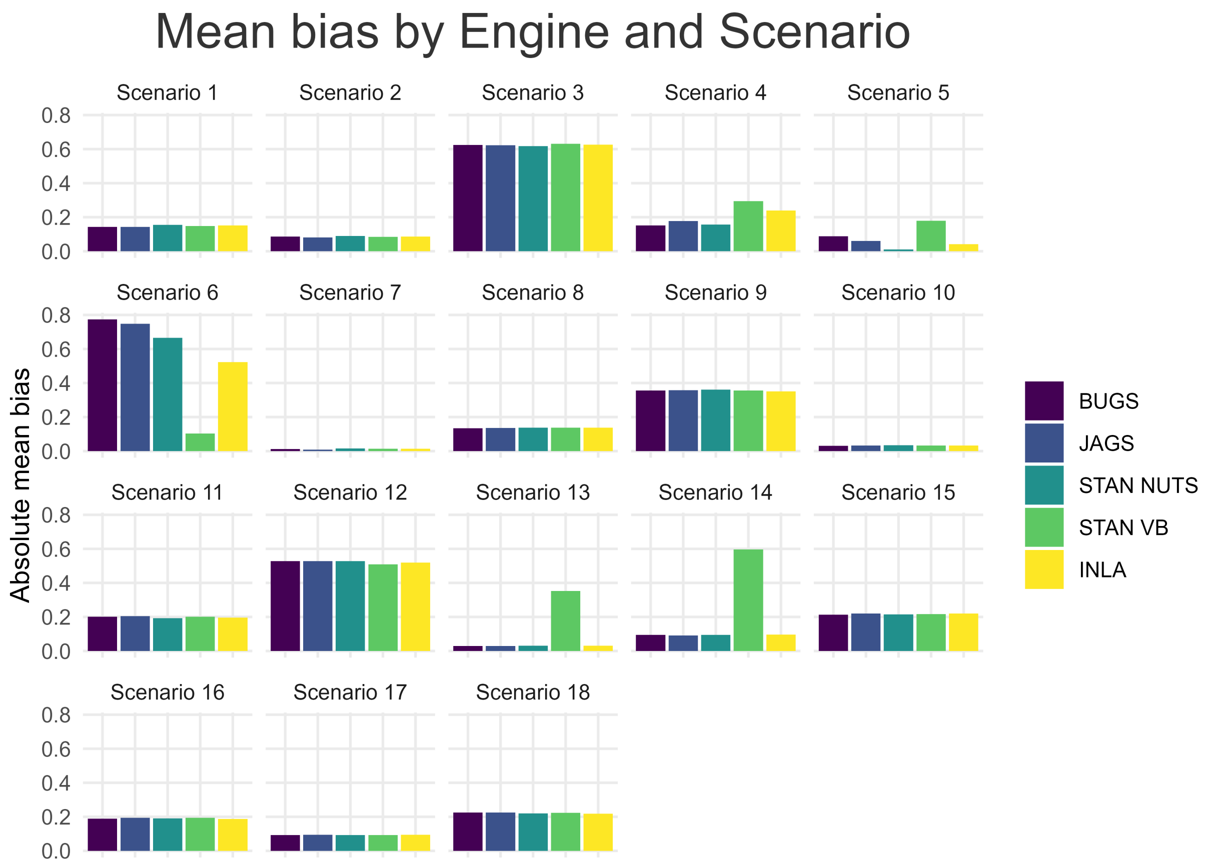


Figure 1: Absolute mean bias for each simulation scenario and engine (averaged over $d$ values).

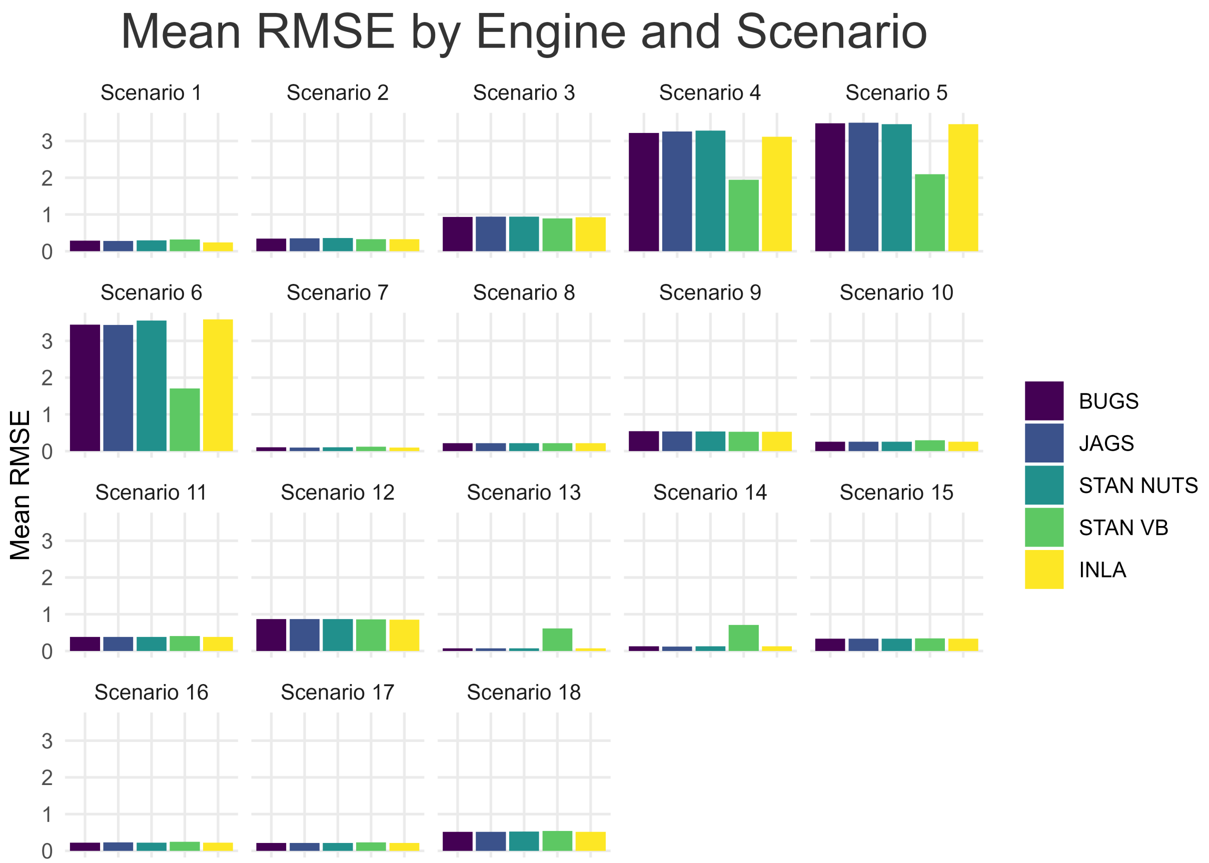


Figure 2: Root mean squared error for each simulation scenario and engine (averaged over $d$ values).

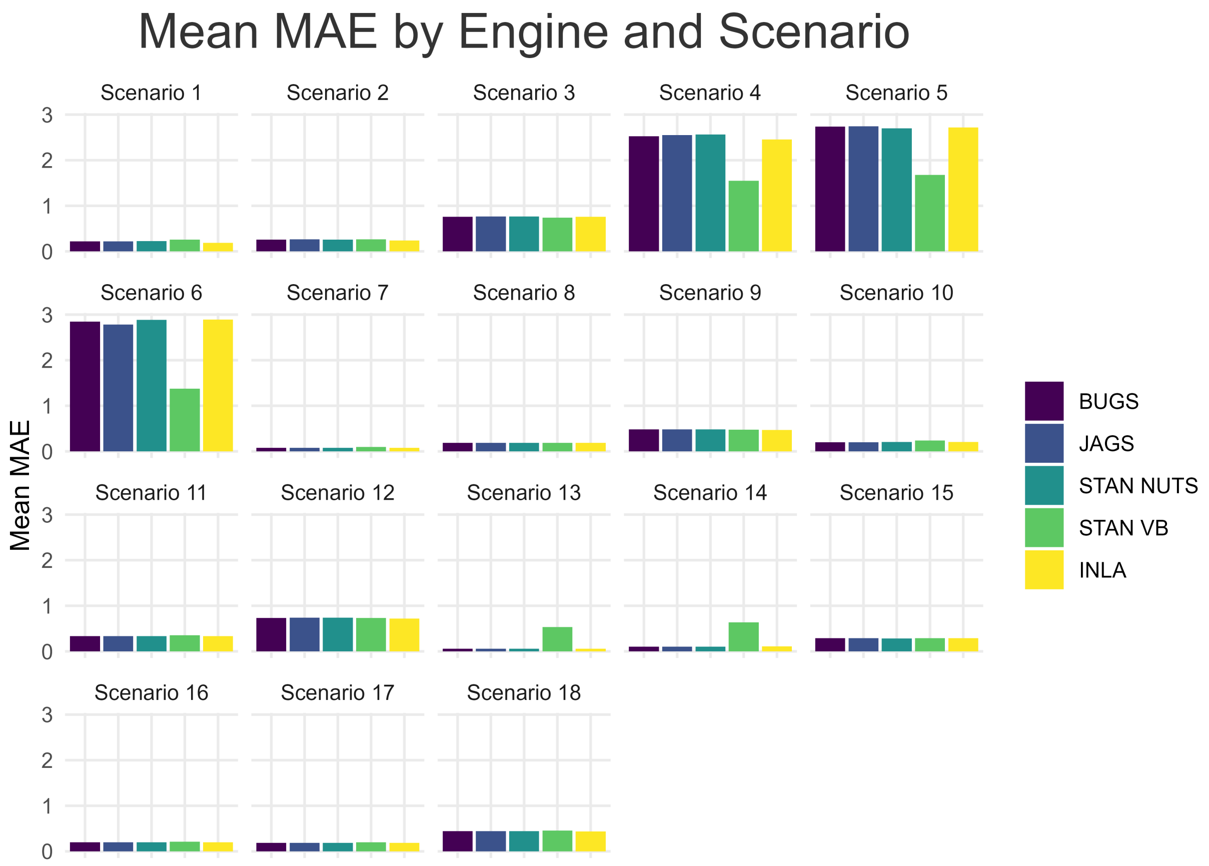


Figure 3: Mean absolute error for each simulation scenario and engine (averaged over $d$ values).

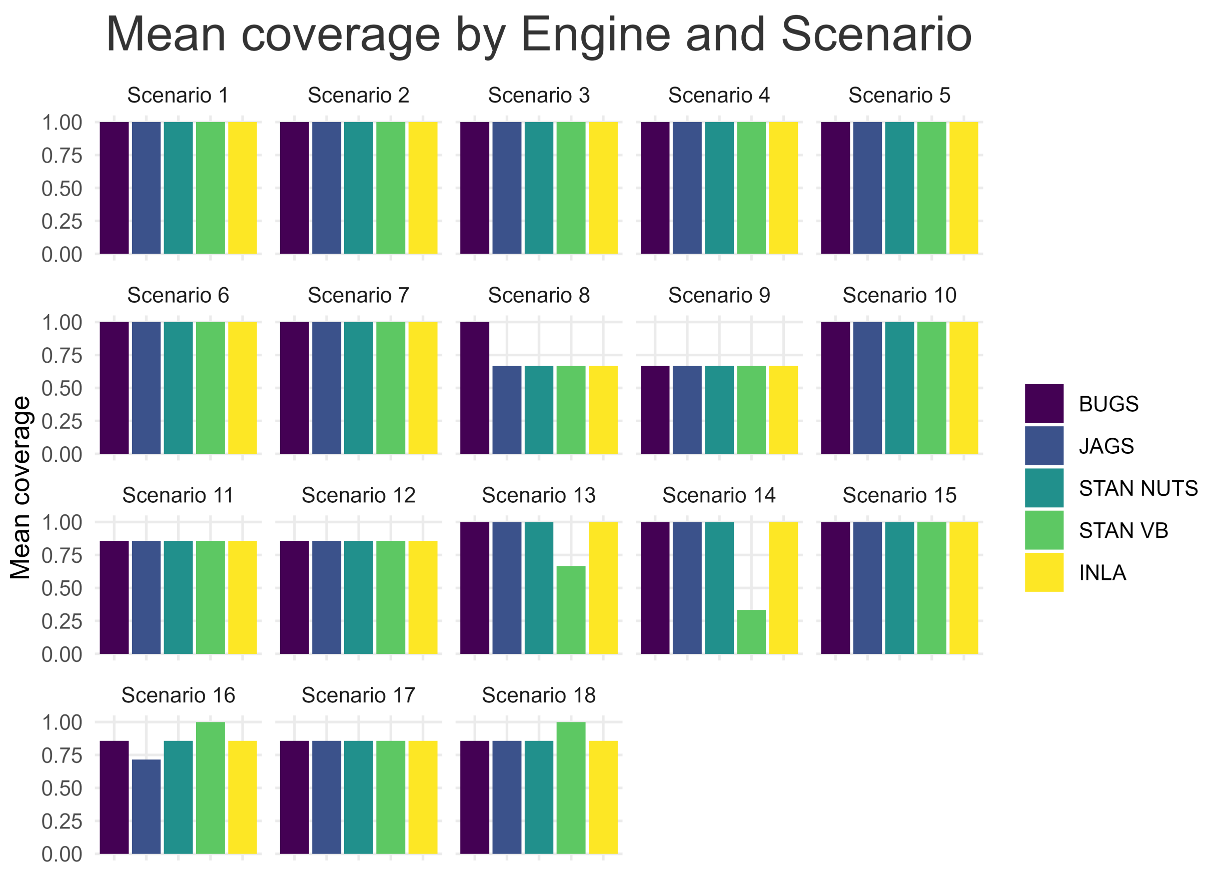


Figure 4: Mean coverage for each simulation scenario and engine (averaged over $d$ values).

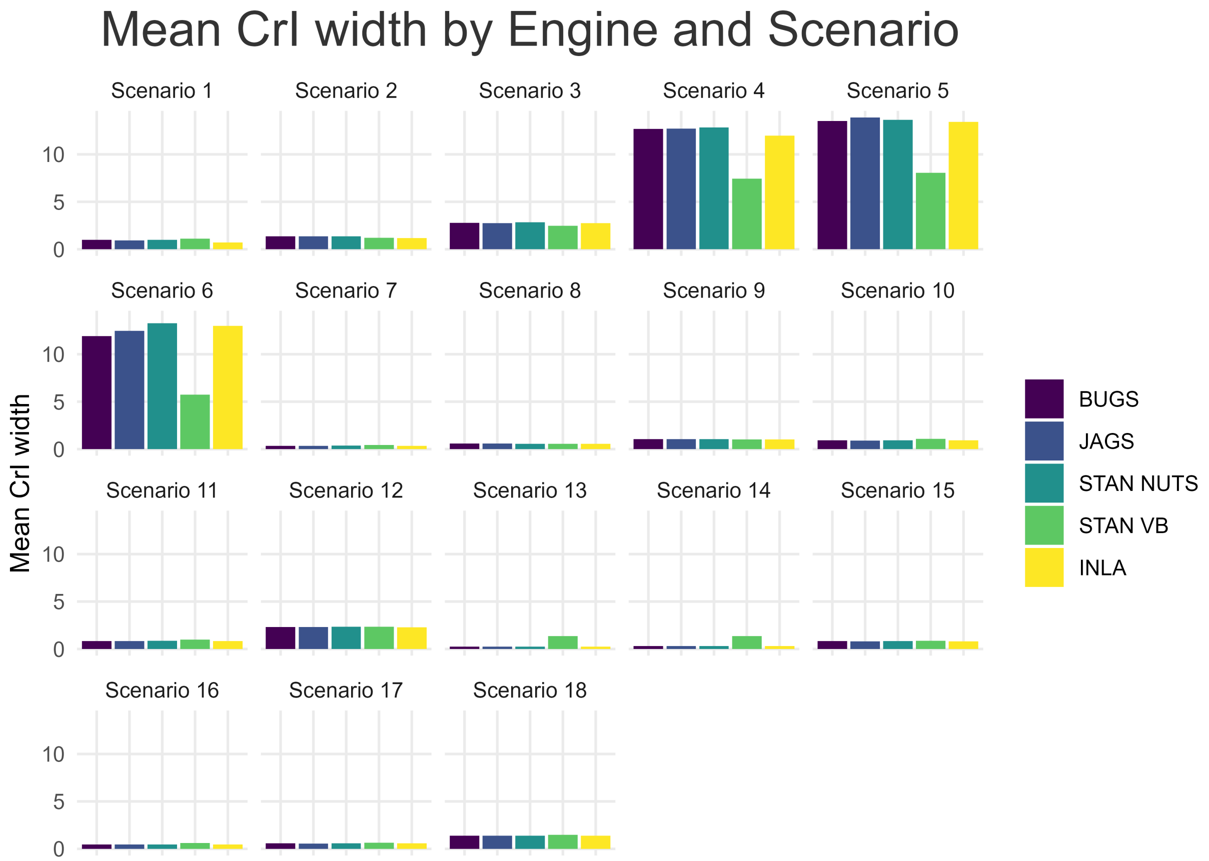


Figure 5: Mean CrI width for each simulation scenario and engine (averaged over $d$ values).

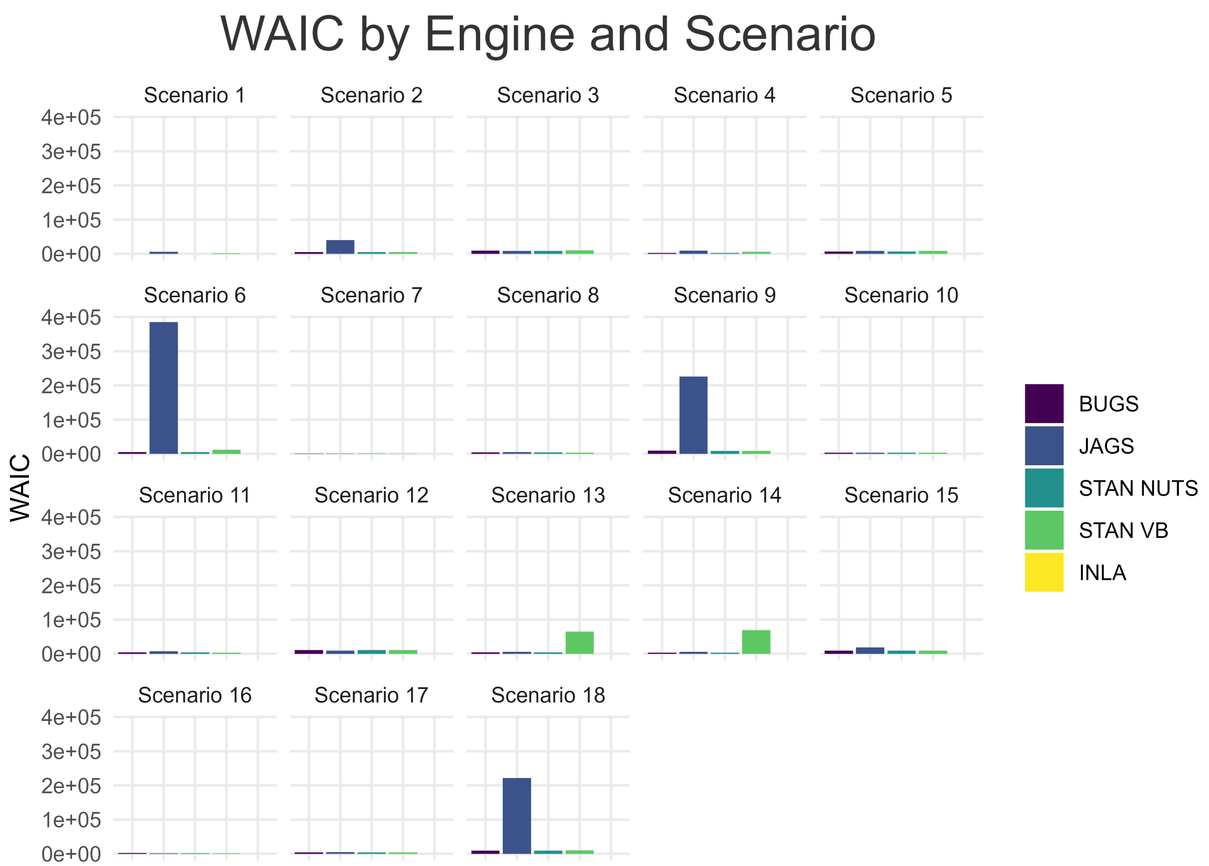


Figure 6: WAIC information criterion for each simulation scenario and engine.

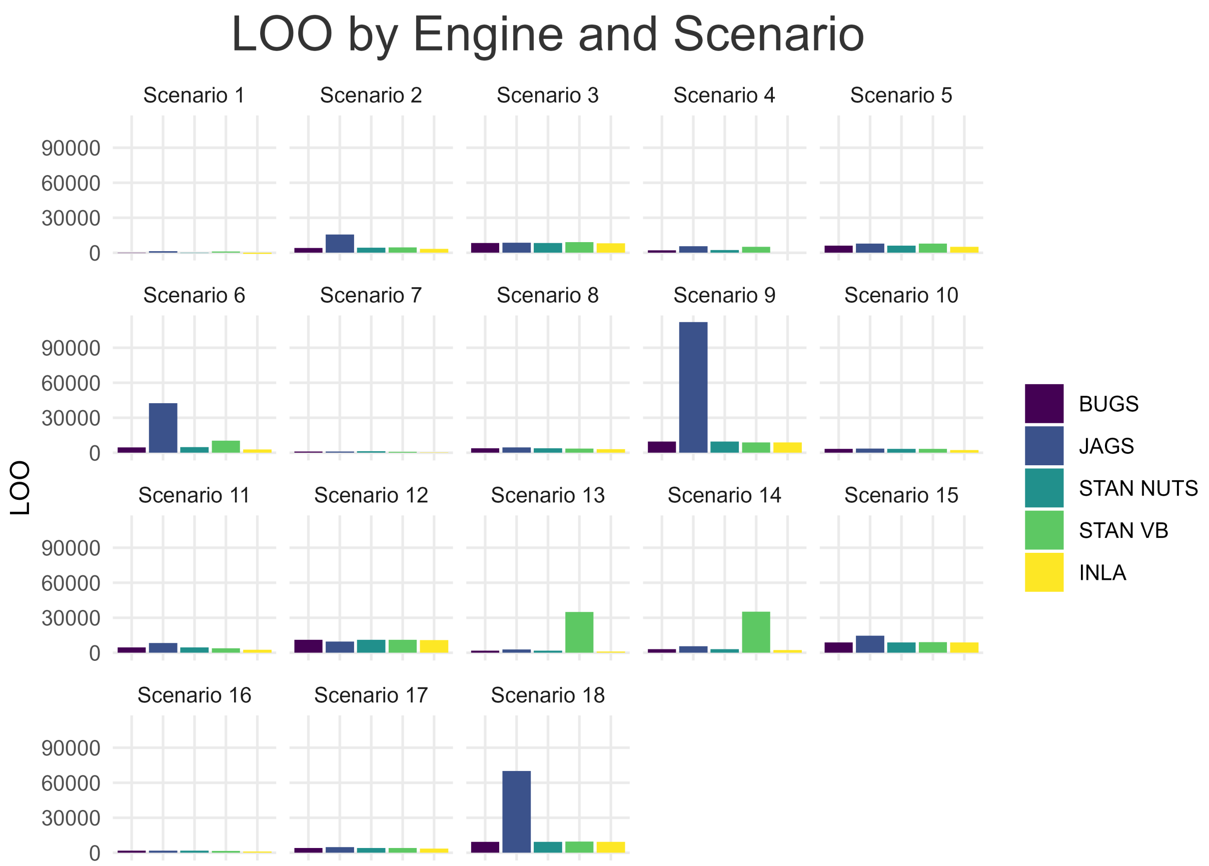


Figure 7: LOO information criterion for each simulation scenario and engine.

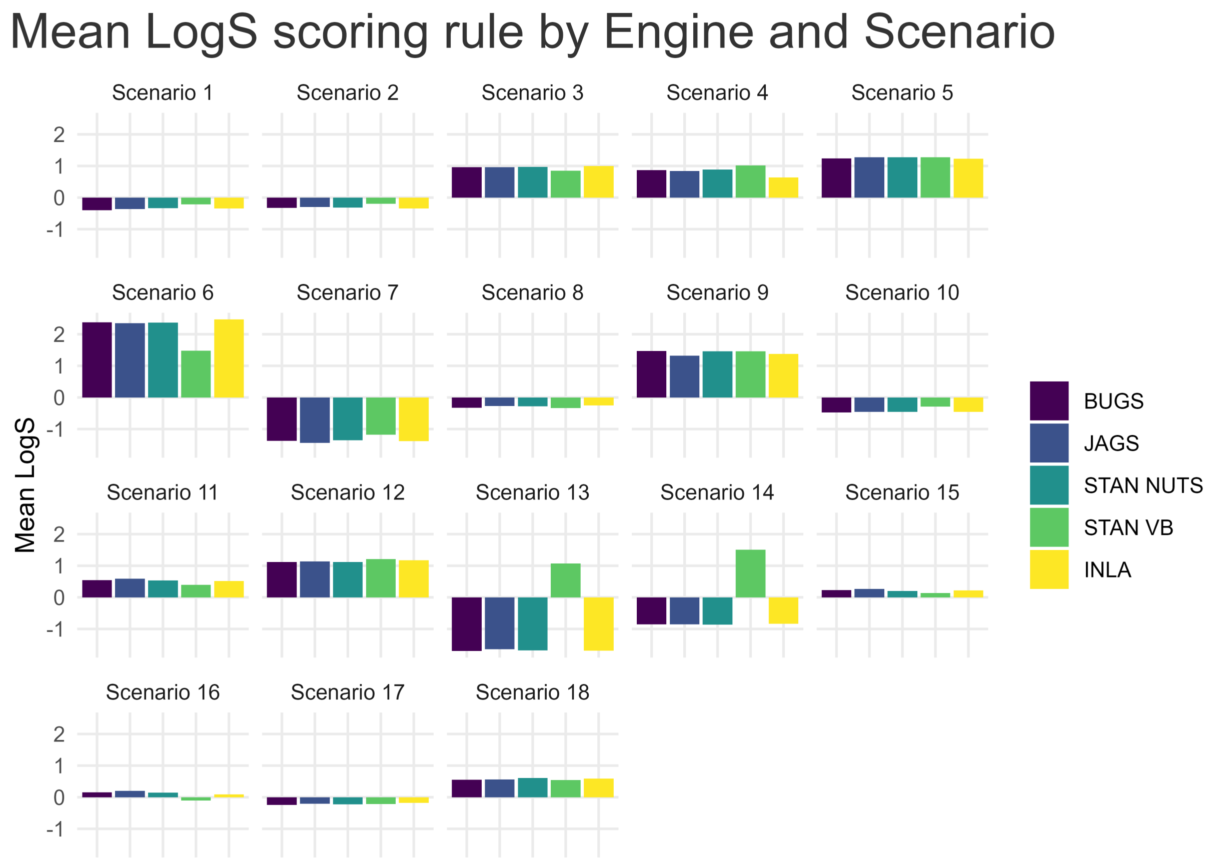


Figure 8: Mean logS scoring rule for each simulation scenario and engine (averaged over $d$ values).

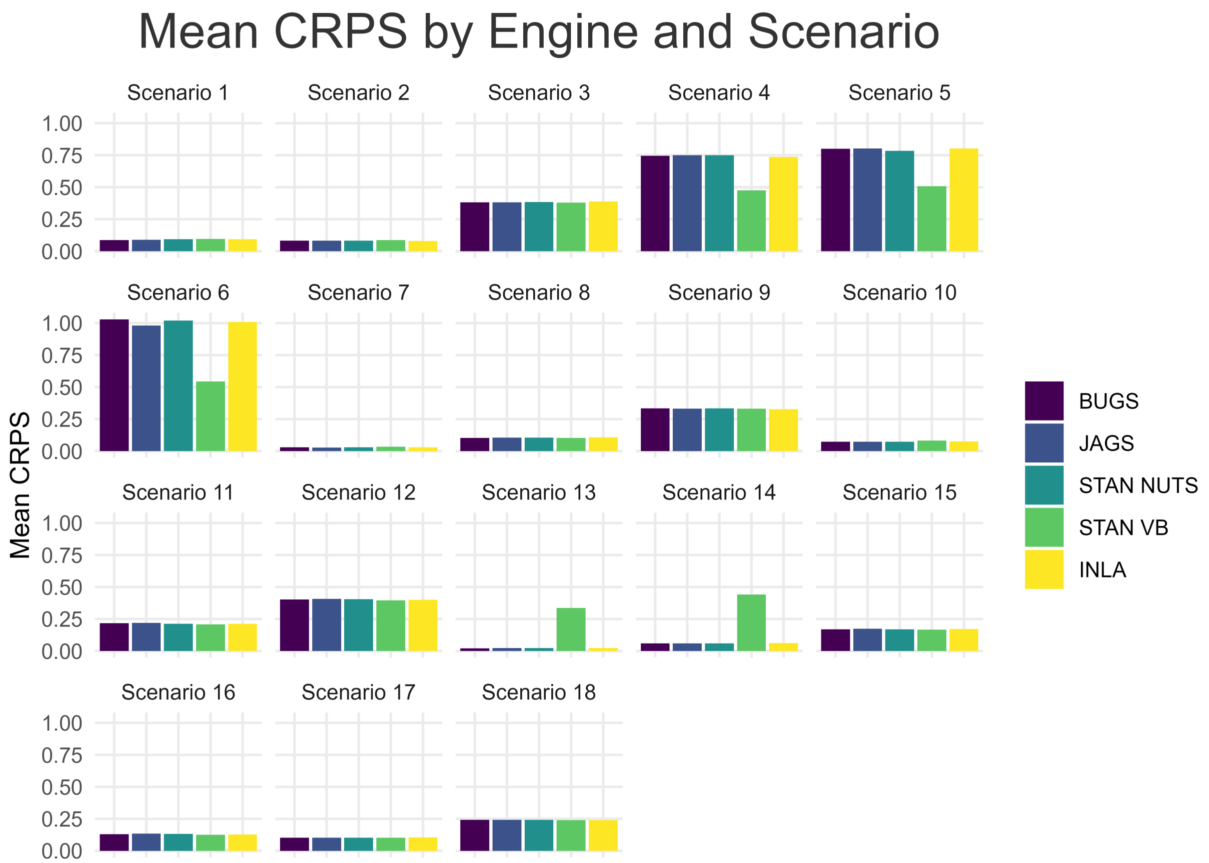


Figure 9: Mean CRPS scoring rule for each simulation scenario and engine (averaged over $d$ values).

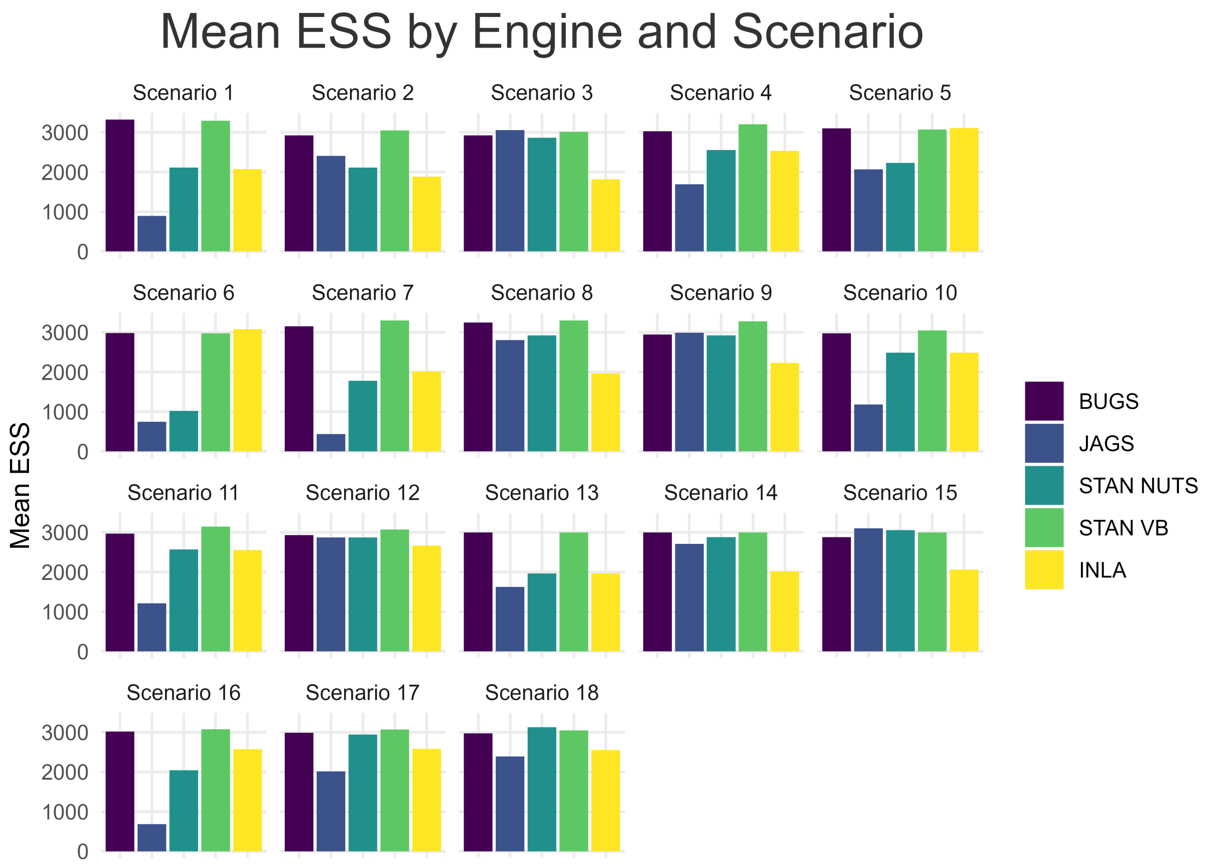


Figure 10: Effective sample size (ESS) for each simulation scenario and engine (averaged over $d$ values).

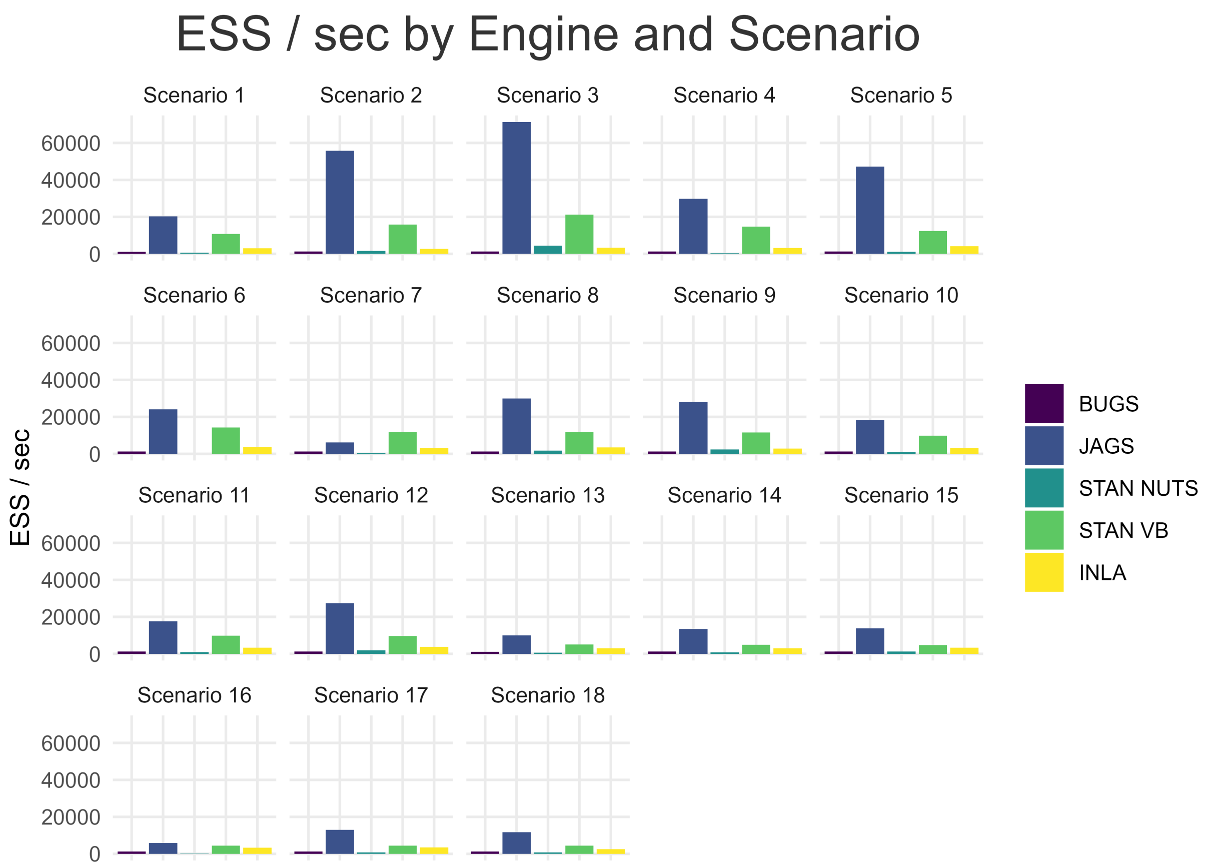


Figure 11: Effective sample size (ESS) per second for each simulation scenario and engine.

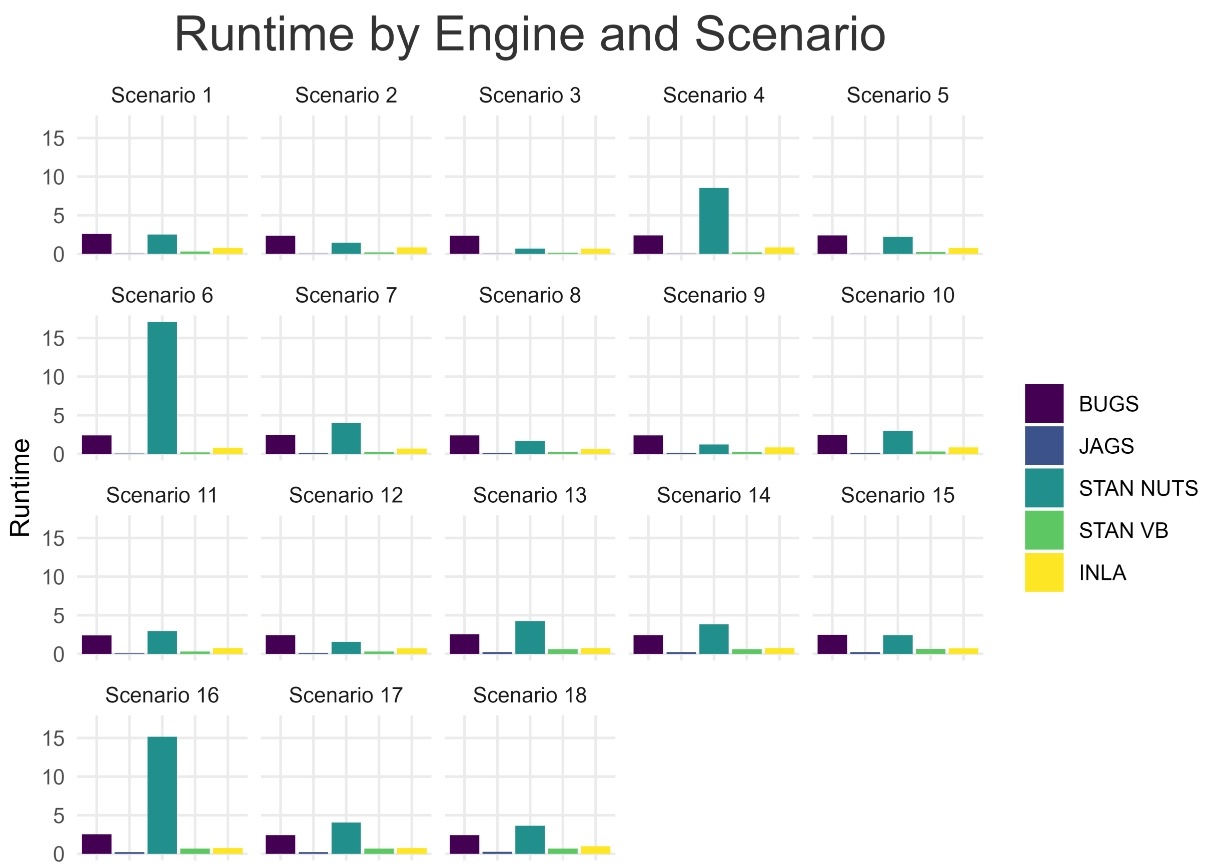


Figure 12: Runtime for each simulation scenario and engine.

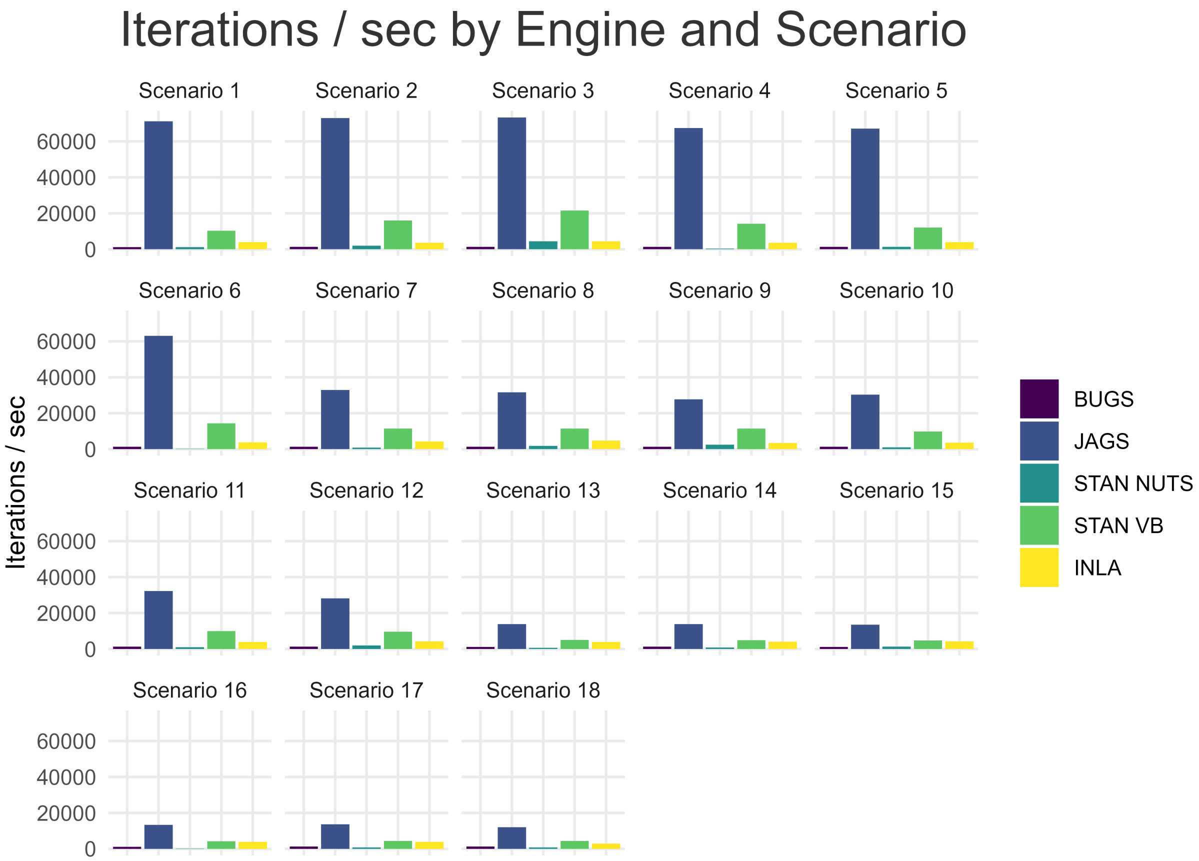


Figure 13: Iterations per second for each simulation scenario and engine.

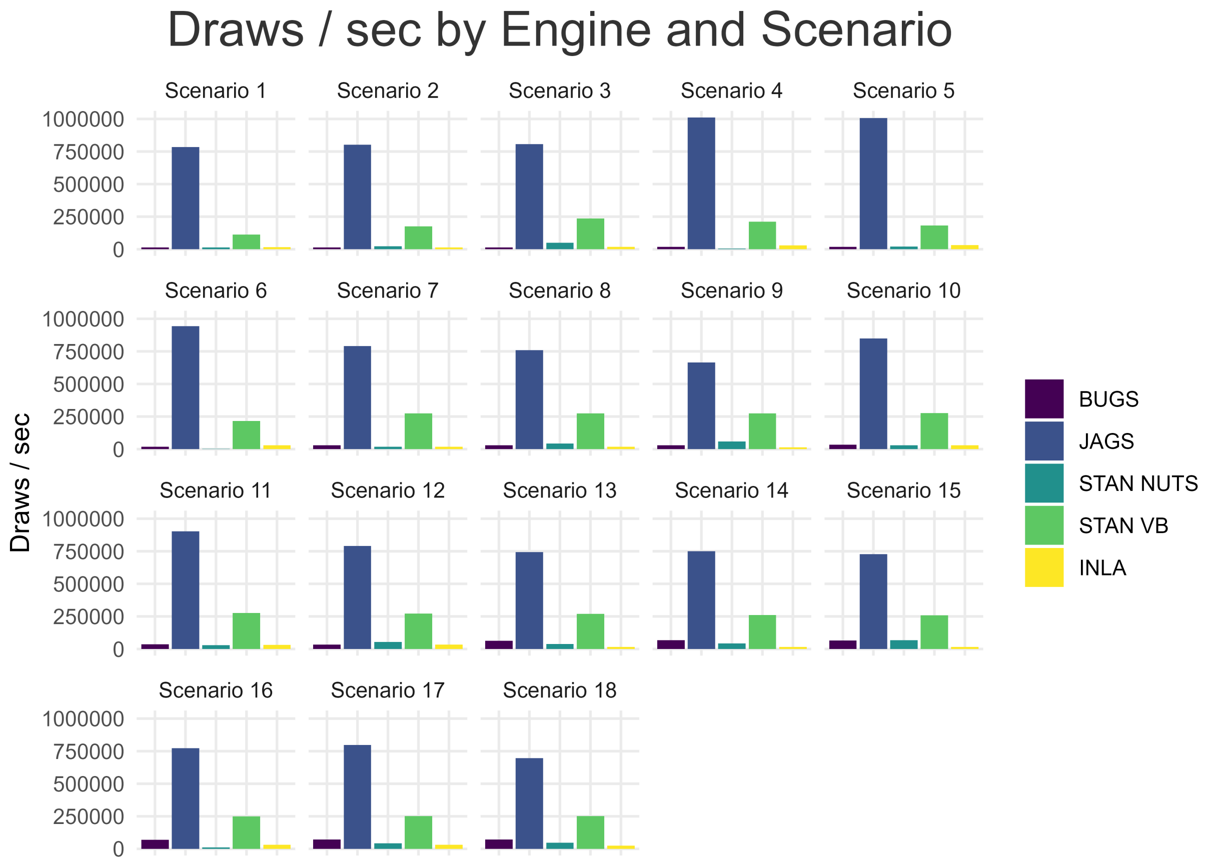


Figure 14: Number of posterior draws per second for each simulation scenario and engine.

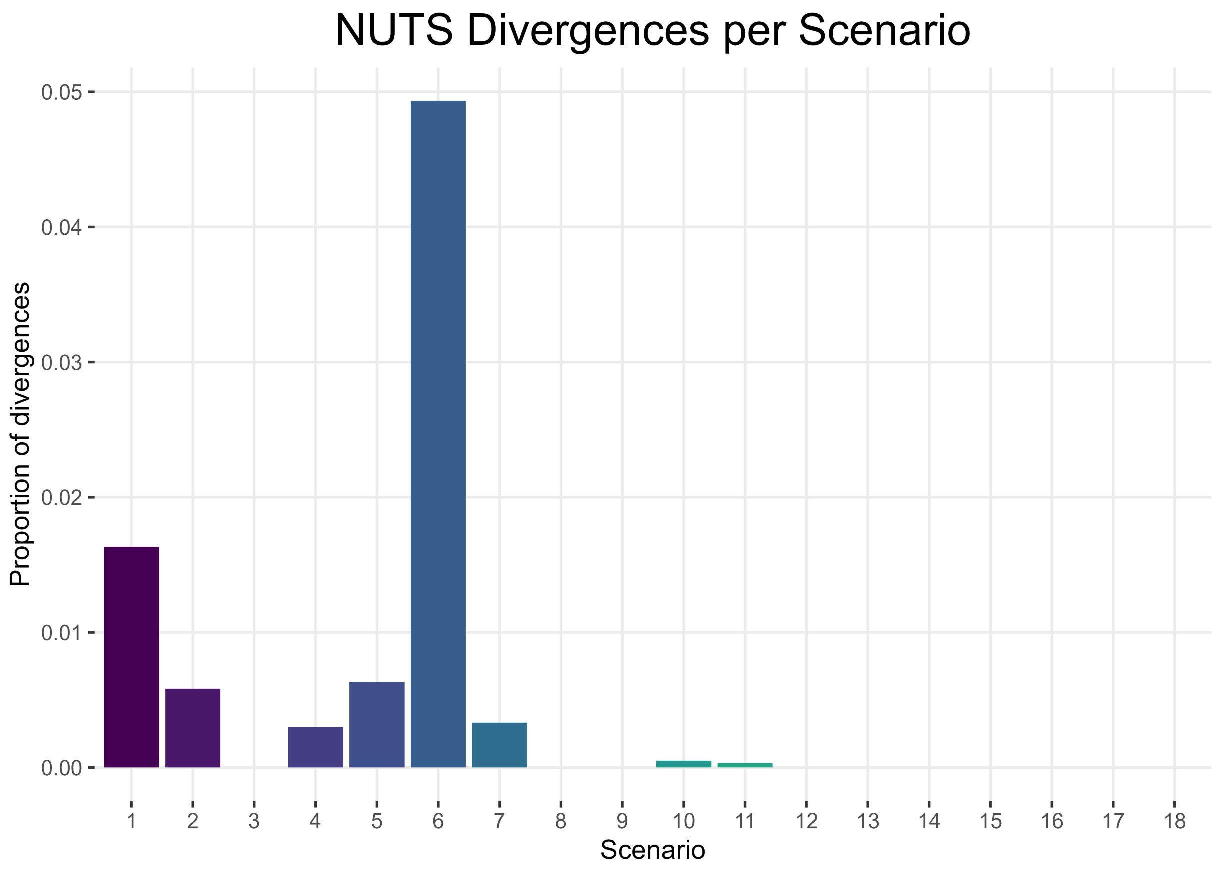


Figure 15: Proportion of divergent transitions for each simulation scenario of the NUTS sampler.

# Web Appendix E. Results on the lung cancer example

More results on the lung cancer example are provided regarding the NMA, decision theory and cost-effectiveness. Unless stated otherwise, the poly-hazard method for extrapolation has been performed and the JAGS engine for meta-analysis is used. The results are based on posterior draws. When an approximation engine is used (ADVI, INLA), parameter draws are simulated by the resulted posterior. In Table 3 a comparison among the engines is provided. JAGS offers the best statistical-computational trade-off, i.e. lowest DIC/WAIC, stable parameter estimates and short runtime. INLA and ADVI are less stable options for this problem. The engines are compared based on typical NMA settings used by practitioners, e.g. NUTS uses more concentrated priors than BUGS/JAGS. For a more comprehensive and fair comparison see the simulation study results. In Table 4 decision-theoretic results are shown. The Pemetrexed treatment is recommended by all methods, except LaEV. The GRADE Working Group method does not recommend any treatment when the cut-off probability exceeds 0.52 (else Pemetrexed is again recommended). In Figures 16 and 17, the probability of each ranking position, SUCRA and cost-effectiveness results are shown. The probabilities per position, when the extrapolation is performed by the M-splines method are shown in Figure 18. The forestplot data comparing the poly-hazard method with the M-splines method are shown in Table 5.

Table 3: Information criteria, effective parameter counts and computation time by engine. The model includes 11 parameters. The best engine is highlighted in bold.

| **Engine** | **AIC** | **BIC** | **DIC** | **DIC$_2$** | **WAIC** | **LOO** | **PSIS–LOO** | $p_D$ | $p_V$ | $p_W$ | **Time (s)** |
|---|---|---|---|---|---|---|---|---|---|---|---|
| BUGS | **63.89** | **63.30** | 48.44 | 48.55 | 50.08 | -26.17 | **25.68** | 3.28 | 3.33 | 3.82 | 5.98 |
| JAGS | 63.90 | 63.30 | 48.35 | **48.55** | **50.04** | -26.08 | 25.91 | 3.23 | 3.33 | 3.81 | **0.05** |
| STAN (NUTS) | 65.96 | 65.37 | 50.89 | 54.56 | 55.58 | -29.75 | 28.83 | 3.46 | 5.30 | 6.26 | 4.33 |
| STAN (ADVI) | 65.95 | 65.36 | 50.47 | 58.52 | 56.35 | **-34.37** | 30.80 | 3.26 | 7.28 | 6.66 | 0.21 |
| INLA | 72.74 | 72.15 | **48.17** | 58.37 | 52.73 | -24.45 | NA | -3.14 | 3.81 | 1.61 | 1.01 |

Table 4: Decision-theoretic quantities for each treatment based on the JAGS posterior samples. The best treatment is highlighted in bold. The top Table holds the results for the posterior mean, probability best, regret and squared regret loss functions. The bottom Table contains all the quantities for construction of the LaEV criterion and the final recommendation.

| **Treatment** | **Posterior Mean** | **Prob. Best** | **Regret** | **Squared Regret** |
|---|---|---|---|---|
| Docetaxel | 0.000 | 0.183 | 2.711 | 14.203 |
| Gefitinib | 0.298 | 0.317 | 2.414 | 13.987 |
| Placebo | -6.430 | 0.007 | 9.142 | 99.566 |
| **Pemetrexed** | **0.814** | **0.493** | **1.897** | **11.464** |

| **Treatment** | $EV_1$ | $EL_1$ | $LaEV_1$ | $EV_2$ | $EL_2$ | $LaEV_2$ | Recommend |
|---|---|---|---|---|---|---|---|
| Docetaxel | 0.000 | 0.000 | 0.000 | 0.000 | 0.000 | 0.000 | TRUE |
| Gefitinib | 0.298 | 0.697 | $-0.399$ | $-0.298$ | 0.503 | 0.205 | FALSE |
| Placebo | $-6.430$ | 6.460 | $-12.890$ | 6.430 | 5.974 | 12.404 | FALSE |
| Pemetrexed | 0.814 | 1.377 | $-0.562$ | $-0.814$ | 1.179 | 0.365 | FALSE |

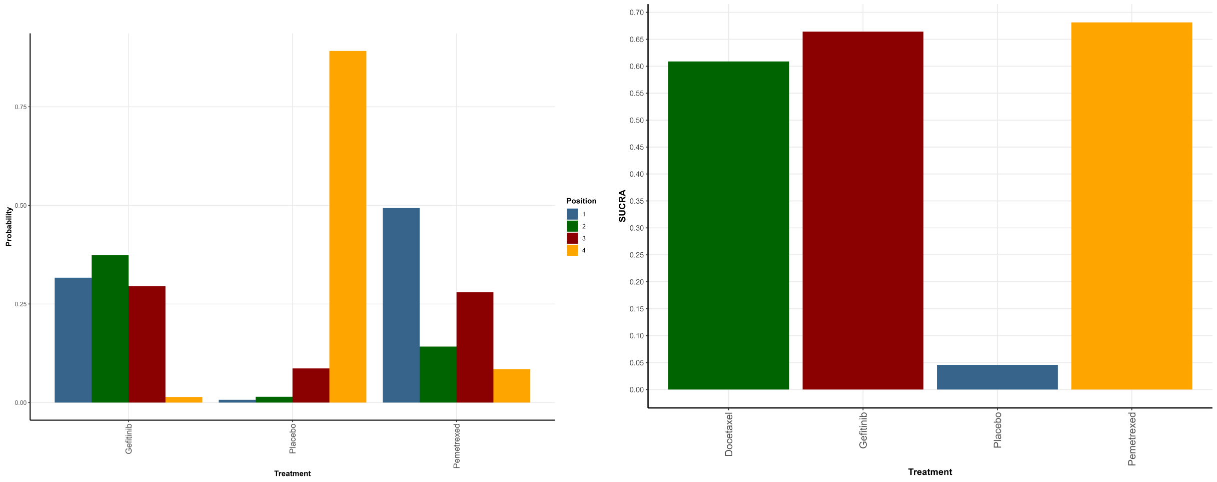


Figure 16: Left: Probability of each treatment being in every ranking position. Right: SUCRA values per treatment. The suggested ranking is Pemetrexed-Gefitinib-Docetaxel-Placebo.

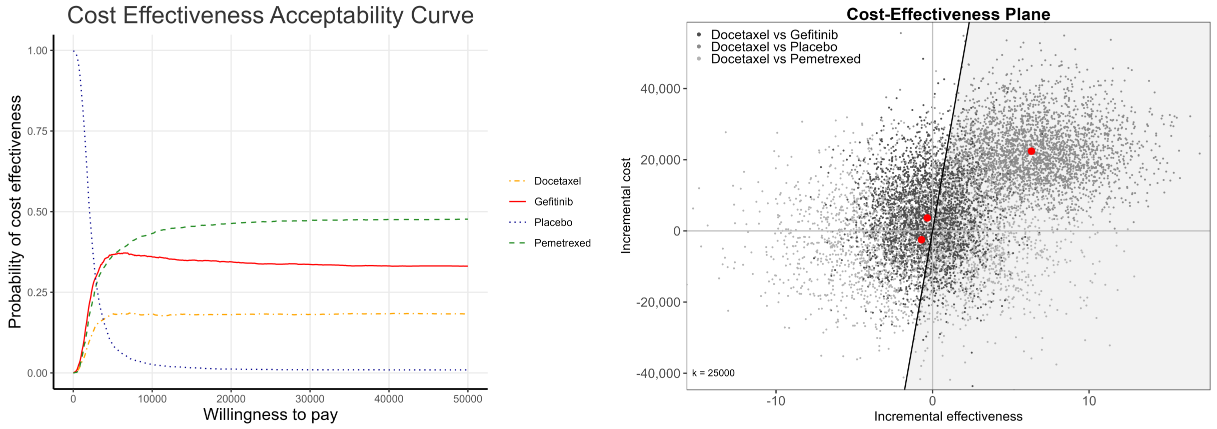


Figure 17: Left: Cost-effectiveness acceptability curves. Probability of cost effectiveness on the y-axis versus willingness to pay parameter on the x-axis. Right: Cost-effectiveness plane. Pemetrexed is the only cost-effective treatment.

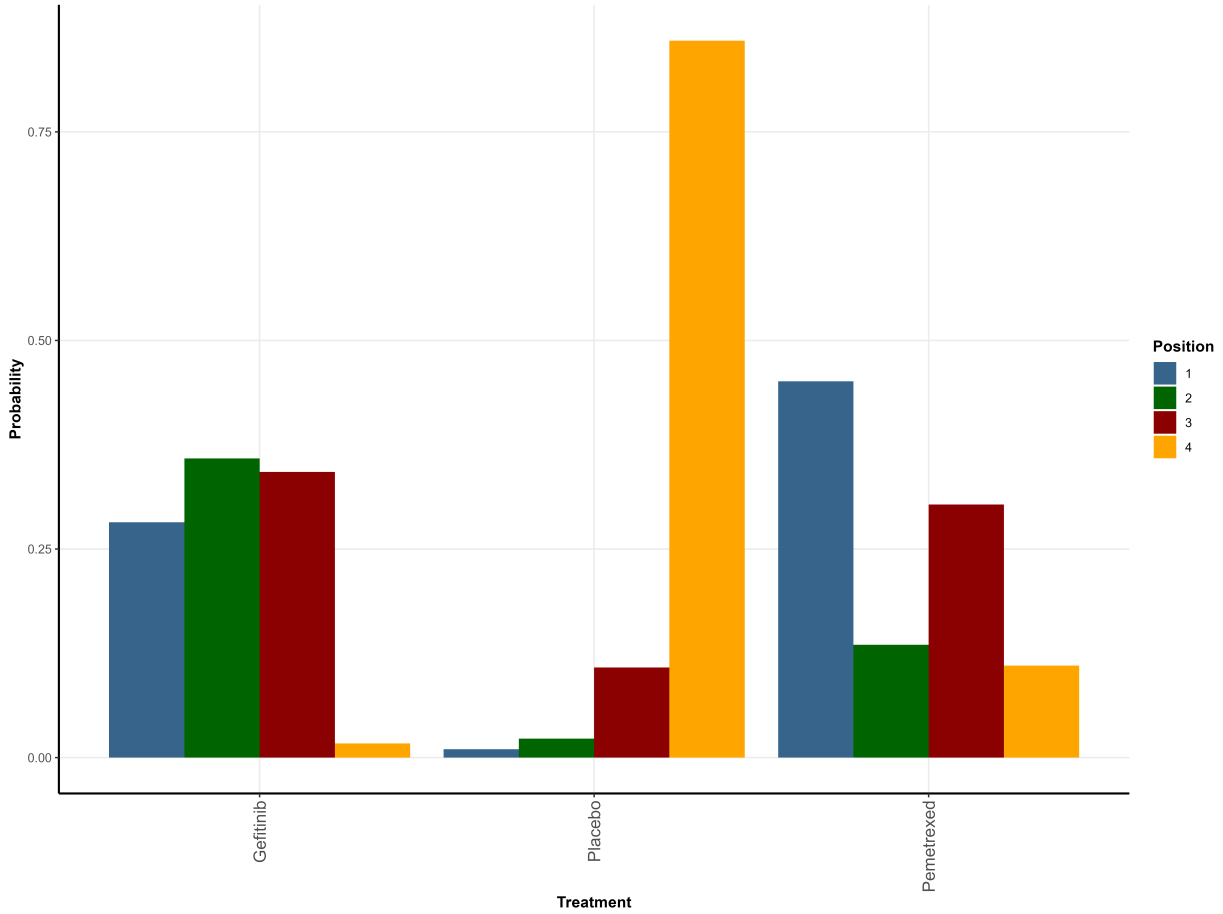


Figure 18: Probability of each ranking position per treatment for the lung cancer application, after fitting the JAGS NMA model on the M-splines-based extrapolations.

Table 5: Data of the forestplot for the lung cancer example presented in the main text.

| Method | Treatment | Mean | Lower | Upper | Rank |
|---|---|---|---|---|---|
| Poly-hazard | Gefitinib | 0.36 | -4.12 | 4.29 | 2 |
| | Placebo | -6.49 | -13.13 | -0.08 | 4 |
| | Pemetrexed | 0.91 | -8.11 | 9.14 | 1 |
| M-splines | Gefitinib | -0.17 | -3.54 | 3.54 | 2 |
| | Placebo | -5.36 | -10.92 | 0.22 | 4 |
| | Pemetrexed | 0.16 | -6.61 | 7.88 | 1 |

# Web Appendix F. Results on the melanoma example

Here, we show more results on the melanoma example. Just as with the lung cancer case, the poly-hazard method for extrapolation and the JAGS engine for meta-analysis are used (unless stated otherwise). The results are based on posterior draws. When an approximation engine is used (ADVI, INLA), parameter draws are simulated by the resulted posterior. In Table 6 a comparison among the engines is provided. JAGS outperforms the other engines, as in the lung cancer example. The engines are compared based on typical NMA settings used by practitioners. In Tables 7 and 8 decision-theoretic results are shown. Nivolumab+Ipilimumab treatment is recommended by all methods, as well as by the GRADE Working Group method with cut-off probability the standard 0.975. In Figure 19, the SUCRA values are shown. In Figure 20, the probability for each position per treatment is shown. The forestplot data comparing the poly-hazard method with the M-splines method are shown in Table 9.

Table 6: Information criteria, effective parameter counts and computation time by engine. The model includes 27 parameters. The best engine is highlighted in bold. Regarding STAN, we tried either the conditional approach of the random effects, or the multivariate and either a centred, or non-centred parametrizations. We write NUTS 1 for 'conditional, centred', NUTS 2 for 'conditional, non-centred', NUTS 3 for 'multivariate, centred', NUTS 4 for 'multivariate non-centred', ADVI 1 for 'conditional centred' and ADVI 2 for 'multivariate centred'. We consider ADVI unreliable, so we exclude it from comparisons.

| **Engine** | **AIC** | **BIC** | **DIC** | **DIC$_2$** | **WAIC** | **LOO** | **PSIS–LOO** | $p_D$ | $p_V$ | $p_W$ | **Time (s)** |
|---|---|---|---|---|---|---|---|---|---|---|---|
| BUGS | 31.03 | 46.28 | 4.99 | 7.23 | 1.90 | **-7.24** | 4.83 | 13.98 | 15.10 | 7.78 | 6.12 |
| JAGS | 31.07 | 46.33 | 4.98 | 9.36 | 1.81 | -6.76 | 4.90 | 13.95 | 16.14 | 7.73 | **0.12** |
| NUTS 1 | 30.45 | 45.70 | 4.36 | **4.22** | 0.17 | -4.70 | **3.22** | 13.95 | 13.88 | 7.07 | 5.97 |
| NUTS 2 | **30.41** | **45.66** | **4.24** | 4.56 | **0.11** | -5.56 | 3.38 | 13.91 | 14.08 | 7.06 | 2.67 |
| NUTS 3 | 30.47 | 45.73 | 4.47 | 4.85 | 0.31 | -4.26 | 3.44 | 14.00 | 14.19 | 7.11 | 4.38 |
| NUTS 4 | 30.53 | 45.78 | 4.58 | 5.18 | 0.76 | -6.64 | 3.69 | 14.03 | 14.33 | 7.34 | 1.87 |
| ADVI 1 | 73010.18 | 73025.43 | 73107.75 | 10856571 | NA | -43769.44 | 3.36 | 75.79 | 5391808 | 1926416 | 1.57 |
| ADVI 2 | 74137.21 | 74152.46 | 74312.87 | 20191372 | NA | -46132.47 | 5.44 | 114.83 | 10058644 | 3191026 | 0.57 |
| INLA | 197.31 | 213.93 | 141.96 | 355.36 | 144.91 | -127.73 | 118.29 | 7.2 | 105.03 | 4.22 | 1.32 |

Table 7: Posterior means, probability of being best, and expected losses under the regret and squared regret functions for each treatment. The best treatment is highlighted in bold.

| **Treatment** | **Posterior Mean** | **Prob. Best** | **Regret** | **Sq. Regret** |
|---|---|---|---|---|
| Dacarbazine | 0.000 | 0.000 | 83.226 | 6972.058 |
| Dabrafenib | 8.426 | 0.000 | 74.800 | 5660.974 |
| Vemurafenib | 5.512 | 0.000 | 77.714 | 6103.744 |
| Nivolumab | 54.832 | 0.000 | 28.394 | 827.788 |
| Ipilimumab | 10.897 | 0.000 | 72.330 | 5243.898 |
| **Nivolumab + Ipilimumab** | **83.226** | **1.000** | **0.000** | **0.000** |
| Cobimetinib + Vemurafenib | 12.798 | 0.000 | 70.428 | 5049.495 |
| Dabrafenib + Trametinib | 14.081 | 0.000 | 69.145 | 4851.327 |
| Ipilimumab + Sargramostim | 22.474 | 0.000 | 60.752 | 3728.860 |
| Pembrolizumab | 33.936 | 0.000 | 49.290 | 2465.308 |
| Tremelimumab | 5.168 | 0.000 | 78.059 | 6162.557 |
| Dacarbazine + Ipilimumab | 14.245 | 0.000 | 68.982 | 4826.105 |
| Dacarbazine + Selumetinib | 2.186 | 0.000 | 81.040 | 6639.070 |

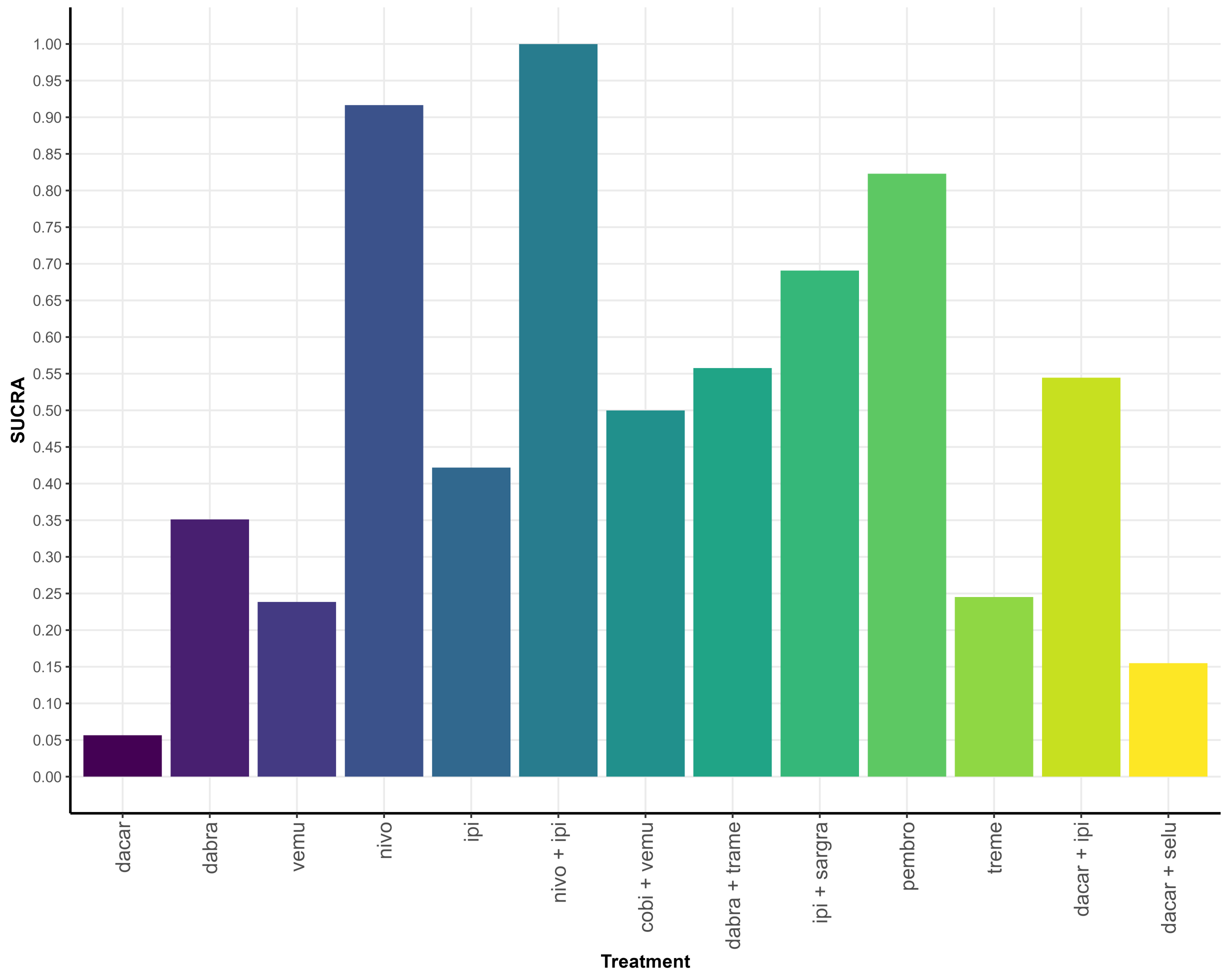


Figure 19: SUCRA values per treatment: Nivolumab+Ipilimumab is suggested.

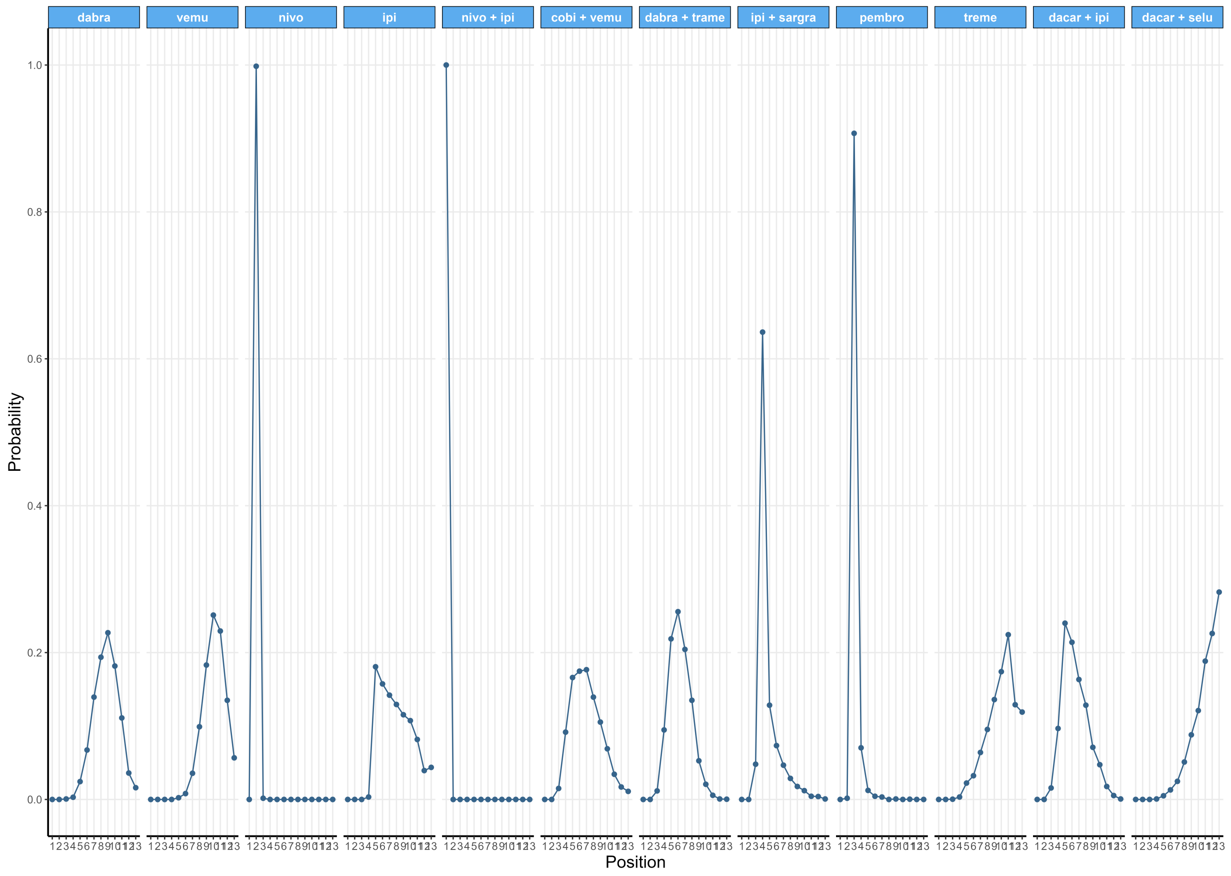


Figure 20: Probability of each ranking position per treatment for the melanoma application, after fitting the JAGS NMA model on the M-splines-based extrapolations.

Table 8: Quantities used in the construction of the LaEV criterion and final recommendation for each treatment.

| **Treatment** | $EV_1$ | $EL_1$ | $LaEV_1$ | $EV_2$ | $EL_2$ | $LaEV_2$ | Recommend |
|---|---|---|---|---|---|---|---|
| Dacarbazine | 0.000 | 0.000 | 0.000 | 83.226 | 82.726 | 165.952 | FALSE |
| Dabrafenib | 8.426 | 0.038 | 8.388 | 74.800 | 74.300 | 149.100 | FALSE |
| Vemurafenib | 5.512 | 0.178 | 5.334 | 77.714 | 77.214 | 154.928 | FALSE |
| Nivolumab | 54.832 | 0.000 | 54.832 | 28.394 | 27.894 | 56.288 | FALSE |
| Ipilimumab | 10.897 | 0.175 | 10.722 | 72.330 | 71.830 | 144.159 | FALSE |
| Nivolumab + Ipilimumab | 83.226 | 0.000 | 83.226 | 0.000 | 0.000 | 0.000 | TRUE |
| Cobimetinib + Vemurafenib | 12.798 | 0.058 | 12.740 | 70.428 | 69.928 | 140.357 | FALSE |
| Dabrafenib + Trametinib | 14.081 | 0.001 | 14.080 | 69.145 | 68.645 | 137.790 | FALSE |
| Ipilimumab + Sargramostim | 22.474 | 0.008 | 22.466 | 60.752 | 60.252 | 121.004 | FALSE |
| Pembrolizumab | 33.936 | 0.000 | 33.936 | 49.290 | 48.790 | 98.080 | FALSE |
| Tremelimumab | 5.168 | 0.357 | 4.810 | 78.059 | 77.559 | 155.617 | FALSE |
| Dacarbazine + Ipilimumab | 14.245 | 0.001 | 14.244 | 68.982 | 68.482 | 137.463 | FALSE |
| Dacarbazine + Selumetinib | 2.186 | 1.062 | 1.124 | 81.040 | 80.540 | 161.581 | FALSE |

Table 9: Data of the forestplot for the melanoma example presented in the main text.

| Method | Treatment | Mean | Lower | Upper | Rank |
|---|---|---|---|---|---|
| Poly-hazard | Dabrafenib | 8.25 | -0.76 | 16.02 | 9 |
| | Vemurafenib | 5.53 | -2.84 | 13.64 | 10 |
| | Nivolumab | 54.85 | 45.79 | 64.73 | 2 |
| | Ipilimumab | 11.10 | -1.70 | 24.42 | 5 |
| | Nivolumab plus Ipilimumab | 83.48 | 70.14 | 96.56 | 1 |
| | Cobimetinib plus Vemurafenib | 12.95 | 0.53 | 26.63 | 6 |
| | Dabrafenib plus Trametinib | 14.13 | 4.19 | 23.61 | 6 |
| | Ipilimumab plus Sargramostim | 22.54 | 6.39 | 39.73 | 4 |
| | Pembrolizumab | 34.33 | 18.36 | 50.48 | 3 |
| | Tremelimumab | 4.99 | -4.70 | 14.34 | 11 |
| | Dacarbazine plus Ipilimumab | 14.21 | 4.71 | 24.35 | 5 |
| | Dacarbazine plus Selumetinib | 2.20 | -7.10 | 11.76 | 13 |
| M-splines | Dabrafenib | 1.03 | -6.12 | 8.65 | 13 |
| | Vemurafenib | 2.44 | -4.93 | 9.97 | 11 |
| | Nivolumab | 26.65 | 18.13 | 35.66 | 3 |
| | Ipilimumab | 17.55 | 6.67 | 30.62 | 5 |
| | Nivolumab plus Ipilimumab | 30.75 | 19.93 | 43.07 | 1 |
| | Cobimetinib plus Vemurafenib | 14.57 | 2.81 | 25.46 | 6 |
| | Dabrafenib plus Trametinib | 8.37 | -0.16 | 16.85 | 7 |
| | Ipilimumab plus Sargramostim | 21.80 | 7.55 | 36.66 | 4 |
| | Pembrolizumab | 28.55 | 13.81 | 43.44 | 2 |
| | Tremelimumab | 5.70 | -2.62 | 14.59 | 9 |
| | Dacarbazine plus Ipilimumab | 8.79 | 0.36 | 17.71 | 7 |
| | Dacarbazine plus Selumetinib | 4.81 | -3.93 | 13.65 | 9 |
